# Supplementary material for: FedNorm: Modality-Based Normalization in Federated Learning for Multi-Modal Liver Segmentation
Source: arXiv:2205.11096 source file (2022-05-23)
Supplement: Supplementary file 1 [file appendix_comparison.tex]

\section{Appendix}\label{sec:appendix-comparison}

\Cref{tab:comparison-non-iid-1-2} shows the comparison on the Non-IID 1 and Non-IID 2 settings based on the
Dice per patient scores. Overall, the federated models show a good performance. However, on the CHAOS19 MR T1 
In-Phase client of the Non-IID 1, the federated models fail because MRI data is underrepresented in this setting.
Nevertheless, the performance of \fednorm is much better than the performances of other FL algorithms.
In general, MRI data is underrepresented in both of these settings, as the volumes contain a low number of slices.
Consequently, the single mode for MRI data normalization of \fednormp is not well trained. Thus, the global model 
of \fednormp shows a poor performance. It can further be noticed that \fednorm is the winning FL algorithm (bold 
highlighting). In the Non-IID 2 setting, the models of \fednorm consistently outperform the local model 
performances on MRI clients, which is not the case for other FL algorithms.
% !TeX root = ../main.tex
% Add the above to each chapter to make compiling the PDF easier in some editors.
\begin{table*}[ht]
	\caption[Comparison: Non-IID 1 and Non-IID 2 Settings]{Comparison on the Non-IID 1 and Non-IID 2 settings. The numbers give the performances of the local models, the centralized model, and the
															federated global models (without refinement at the clients) on the test set of each client. The performances are reported with Dice per
															patient and are given by mean (median) and standard deviation. Additionally, the RI according to \Cref{eqn:relative-improvement} is computed
															for the mean Dice per patient of the models from the FL algorithms and the centralized model over the local model
															performance. Hence, the RI is not reported for the local models. The best score from the federated models per client is highlighted
															in bold. A star ($^\ast$) before/behind (Non-IID 1/2 setting) the model name indicates that the results are statistically significant
															with a $p$-value $\leq 0.05$ using the unpaired two-sided t-test on the Dice per patient scores from the local model
															and the respective federated/centralized model.}\label{tab:comparison-non-iid-1-2}
	\centering
	\begin{adjustbox}{max width=\textwidth, max height=0.44\textheight}
		\begin{tabular}{c c c c c c}
			\toprule
			\multirow{2}{*}{\shortstack{\textbf{Client}\\\textbf{(Modality)}}}& \multirow{2}{*}{\textbf{Algorithms}}& \textbf{Non-IID 1}								& \textbf{RI (Non-IID 1)}								& \textbf{Non-IID 2}										& \textbf{RI (Non-IID 2)}									\\
																			&										& \textbf{Dice per Patient} $\boldsymbol{\uparrow}$	& \textbf{[\%]} $\boldsymbol{\uparrow}$					& \textbf{Dice per Patient} $\boldsymbol{\uparrow}$			& \textbf{[\%]} $\boldsymbol{\uparrow}$						\\
			\midrule
			\multirow{8}{*}{\shortstack{Multi-Atlas\\(CT)}}					& Local									& $0.867\,(0.889) \pm 0.061$						& -														& $0.867\,(0.889) \pm 0.061$								& -															\\
																			  \cdashline{3-6}
																			& FedAvg$^\ast$							& $0.871\,(0.878) \pm 0.072$						& 0.461													& $0.904\,(0.910) \pm 0.045$								& 4.268														\\
																			& $^\ast$FedAvgM$^\ast$					& $0.724\,(0.741) \pm 0.090$						& -16.494												& $0.574\,(0.584) \pm 0.164$								& -33.795													\\
																			& $^\ast$FedVC$^\ast$					& $0.826\,(0.822) \pm 0.046$						& -4.729												& $0.488\,(0.472) \pm 0.144$								& -43.714													\\
																			& $^\ast$SiloBN							& $0.932\,(0.943) \pm 0.028$						& 7.497													& $0.825\,(0.853) \pm 0.077$								& -4.844													\\
																			& $^\ast$FedBN$^\ast$					& $\boldsymbol{0.934\,(0.945) \pm 0.026}$			& $\boldsymbol{7.728}$									& $0.915\,(0.937) \pm 0.040$								& 5.536														\\
																			& $^\ast$FedNorm$^\ast$					& $0.905\,(0.929) \pm 0.049$						& 4.383													& $\boldsymbol{0.923\,(0.931) \pm 0.027}$					& $\boldsymbol{6.459}$										\\
																			& FedNorm+								& $0.871\,(0.878) \pm 0.074$						& 0.461													& $0.831\,(0.861) \pm 0.088$								& -4.152													\\
																			  \cdashline{3-6}
																			& $^\ast$Centralized$^\ast$				& $0.933\,(0.944) \pm 0.030$						& 7.612													& $0.937\,(0.947) \pm 0.024$								& 8.074														\\
			\midrule
			\multirow{8}{*}{\shortstack{3D-IRCADb\\(CT)}}					& Local									& $0.908\,(0.914) \pm 0.026$						& -														& $0.908\,(0.914) \pm 0.026$								& -															\\
																			  \cdashline{3-6}
																			& FedAvg$^\ast$							& $0.925\,(0.934) \pm 0.027$						& 1.872													& $0.942\,(0.942) \pm 0.022$								& 3.744														\\
																			& $^\ast$FedAvgM						& $0.323\,(0.240) \pm 0.238$						& -64.427												& $0.852\,(0.881) \pm 0.072$								& -6.167													\\
																			& FedVC$^\ast$							& $0.888\,(0.899) \pm 0.030$						& -2.203												& $0.817\,(0.841) \pm 0.051$								& -10.022													\\
																			& $^\ast$SiloBN$^\ast$					& $0.950\,(0.953) \pm 0.015$						& 4.626													& $0.950\,(0.952) \pm 0.017$								& 4.626														\\
																			& $^\ast$FedBN$^\ast$					& $\boldsymbol{0.955\,(0.951) \pm 0.016}$			& $\boldsymbol{5.176}$									& $\boldsymbol{0.960\,(0.959) \pm 0.012}$					& $\boldsymbol{5.727}$										\\
																			& $^\ast$FedNorm$^\ast$					& $0.942\,(0.948) \pm 0.024$						& 3.744													& $\boldsymbol{0.960\,(0.959) \pm 0.011}$					& $\boldsymbol{5.727}$										\\
																			& $^\ast$FedNorm+$^\ast$				& $0.940\,(0.947) \pm 0.029$						& 3.524													& $0.942\,(0.949) \pm 0.019$								& 3.744														\\
																			  \cdashline{3-6}
																			& $^\ast$Centralized$^\ast$				& $0.948\,(0.957) \pm 0.024$						& 4.405													& $0.944\,(0.951) \pm 0.027$								& 3.965														\\
			\midrule
			\multirow{8}{*}{\shortstack{SLIVER07\\(CT)}}					& Local									& $0.903\,(0.907) \pm 0.075$						& -														& $0.903\,(0.907) \pm 0.075$								& -	 														\\
																			  \cdashline{3-6}
																			& FedAvg								& $0.908\,(0.932) \pm 0.086$						& 0.554													& $0.841\,(0.924) \pm 0.251$								& -6.866													\\
																			& $^\ast$FedAvgM						& $0.742\,(0.749) \pm 0.061$						& -17.829												& $0.842\,(0.865) \pm 0.072$								& -6.755													\\
																			& FedVC$^\ast$							& $0.872\,(0.900) \pm 0.102$						& -3.433												& $0.761\,(0.799) \pm 0.147$								& -15.725													\\
																			& SiloBN								& $0.923\,(0.936) \pm 0.052$						& 2.215													& $0.913\,(0.941) \pm 0.071$								& 1.107														\\
																			& FedBN									& $0.920\,(0.930) \pm 0.053$						& 1.883													& $0.932\,(0.941) \pm 0.047$								& 3.212														\\
																			& FedNorm								& $\boldsymbol{0.940\,(0.954) \pm 0.056}$			& $\boldsymbol{4.097}$									& $0.914\,(0.944) \pm 0.096$								& 1.218														\\
																			& FedNorm+								& $0.935\,(0.941) \pm 0.053$						& 3.544													& $\boldsymbol{0.936\,(0.946) \pm 0.040}$					& $\boldsymbol{3.654}$										\\
																			  \cdashline{3-6}
																			& Centralized							& $0.922\,(0.944) \pm 0.084$						& 2.104													& $0.906\,(0.948) \pm 0.104$								& 0.332														\\
			\midrule
			\multirow{8}{*}{\shortstack{CHAOS19 MR\\T1 In-Phase\\(MRI)}}	& Local									& $0.724\,(0.825) \pm 0.287$						& -														& $0.724\,(0.825) \pm 0.287$								& -	 														\\
																			  \cdashline{3-6}
																			& $^\ast$FedAvg							& $0.106\,(0.060) \pm 0.119$						& -85.359												& $0.431\,(0.495) \pm 0.285$								& -40.47													\\
																			& $^\ast$FedAvgM						& $0.021\,(0.004) \pm 0.032$						& -97.099												& $0.638\,(0.771) \pm 0.289$								& -11.878													\\
																			& $^\ast$FedVC							& $0.090\,(0.040) \pm 0.124$						& -87.569												& $0.650\,(0.788) \pm 0.296$								& -10.221													\\
																			& $^\ast$SiloBN							& $0.189\,(0.079) \pm 0.252$						& -73.895												& $0.583\,(0.750) \pm 0.302$								& -19.475													\\
																			& $^\ast$FedBN$^\ast$					& $0.180\,(0.023) \pm 0.304$						& -75.138												& $0.194\,(0.046) \pm 0.302$								& -73.204													\\
																			& FedNorm								& $\boldsymbol{0.469\,(0.511) \pm 0.231}$			& $\boldsymbol{-35.221}$								& $\boldsymbol{0.791\,(0.810) \pm 0.104}$					& $\boldsymbol{9.254}$										\\
																			& $^\ast$FedNorm+$^\ast$				& $0.067\,(0.043) \pm 0.075$						& -90.746												& $0.230\,(0.196) \pm 0.215$								& -68.232													\\
																			  \cdashline{3-6}
																			& Centralized							& $0.618\,(0.739) \pm 0.329$						& -14.641												& $0.712\,(0.896) \pm 0.334$								& -1.657													\\
			\midrule
			\multirow{8}{*}{\shortstack{CHAOS19 MR\\T1 Out-Phase\\(MRI)}}	& Local									& -													& -														& $0.750\,(0.795) \pm 0.138$								& -	 														\\
																			  \cdashline{3-6}
																			& FedAvg$^\ast$							& \multirow{7}{*}{-}								& \multirow{7}{*}{-}									& $0.467\,(0.553) \pm 0.270$								& -37.733													\\
																			& FedAvgM								& 													& 														& $0.700\,(0.791) \pm 0.213$								& -6.667													\\
																			& FedVC									& 													& 														& $0.673\,(0.788) \pm 0.291$								& -10.267													\\
																			& SiloBN								& 													& 														& $0.686\,(0.740) \pm 0.237$								& -8.533													\\
																			& FedBN									& 													& 														& $0.457\,(0.610) \pm 0.381$								& -39.067													\\
																			& FedNorm								& 													& 														& $\boldsymbol{0.755\,(0.767) \pm 0.100}$					& $\boldsymbol{0.667}$										\\
																			& FedNorm+$^\ast$						&													&														& $0.253\,(0.173) \pm 0.265$								& -66.267													\\
																			  \cdashline{3-6}
																			& Centralized							& -													& -														& $0.729\,(0.858) \pm 0.315$								& -2.8														\\
			\midrule
			\multirow{8}{*}{\shortstack{CHAOS19 MR\\T1 Water\\(MRI)}}		& Local									& -													& -														& $0.646\,(0.760) \pm 0.266$								& -	 														\\
																			  \cdashline{3-6}
																			& FedAvg								& \multirow{7}{*}{-}								& \multirow{7}{*}{-}									& $0.451\,(0.530) \pm 0.291$								& -30.186													\\
																			& FedAvgM								& 													& 														& $0.700\,(0.809) \pm 0.254$								& 8.359														\\
																			& FedVC									& 													& 														& $0.690\,(0.821) \pm 0.302$								& 6.811														\\
																			& SiloBN								& 													& 														& $0.717\,(0.742) \pm 0.185$								& 10.991													\\
																			& FedBN									& 													& 														& $0.533\,(0.647) \pm 0.350$								& -17.492													\\
																			& FedNorm								& 													& 														& $\boldsymbol{0.799\,(0.808) \pm 0.090}$					& $\boldsymbol{23.684}$										\\
																			& FedNorm+$^\ast$						&													&														& $0.288\,(0.172) \pm 0.318$								& -55.418													\\
																			  \cdashline{3-6}
																			& Centralized							& -													& -														& $0.738\,(0.891) \pm 0.316$								& 14.241													\\
			\bottomrule
		\end{tabular}
	\end{adjustbox}
\end{table*}
